# Supplementary material for: UNICORN on RAINBOW: A Universal Commonsense Reasoning Model on a New Multitask Benchmark
Source: arXiv:2103.13009 source file (2021-03-24)
Supplement: Supplementary file 1 [file all.multiset_learning-curves.tex]

\begin{tabular}{llrrrrrrrrrr}
\toprule
 & &\multicolumn{10}{c}{\small{Size}}\\ \cline{3-12}
model & transfer &  \small{4} &  \small{10} &  \small{30} &  \small{91} &  \small{280} &  \small{865} &  \small{2667} &  \small{5334} &  \small{8000} &  \small{9741} \\
\midrule
\multirow{3}{*}{base} & fine-tune &       37.5 &        47.1 &        46.5 &        47.9 &         49.2 &         51.0 &          55.1 &          59.2 &          59.9 &          60.6 \\
      & multitask &       36.4 &        47.7 &        46.9 &        48.9 &         49.2 &         52.7 &          55.4 &          58.3 &          59.5 &          60.0 \\
      & sequential &       38.4 &        45.4 &        45.6 &        48.1 &         50.2 &         52.7 &          56.1 &          59.7 &          61.6 &          61.6 \\
\cline{1-12}
\multirow{3}{*}{large} & fine-tune &       47.4 &        64.0 &        63.8 &        63.0 &         65.7 &         66.5 &          68.8 &          71.6 &          71.8 &          72.6 \\
      & multitask &       41.7 &        63.2 &        63.7 &        63.9 &         65.7 &         66.7 &          68.3 &          71.8 &          72.1 &          73.0 \\
      & sequential &       59.5 &        63.3 &        63.0 &        64.0 &         65.9 &         68.1 &          69.8 &          72.9 &          73.1 &          72.6 \\
\cline{1-12}
\multirow{3}{*}{small} & fine-tune &       26.3 &        30.9 &        30.3 &        27.7 &         29.7 &         31.1 &          33.5 &          36.6 &          37.8 &          40.2 \\
      & multitask &       26.3 &        30.7 &        29.7 &        28.9 &         29.9 &         31.7 &          33.0 &          36.6 &          40.5 &          40.1 \\
      & sequential &       25.1 &        28.7 &        29.1 &        27.8 &         29.8 &         31.0 &          32.7 &          38.0 &          39.3 &          41.0 \\
\bottomrule
\end{tabular}
