# Supplementary material for: UNICORN on RAINBOW: A Universal Commonsense Reasoning Model on a New Multitask Benchmark
Source: arXiv:2103.13009 source file (2021-03-24)
Supplement: Supplementary file 2 [file all.single-task_learning-curves.tex]

\begin{tabular}{lrrrrrrrrrr}
\toprule
 &\multicolumn{10}{c}{\small{Size}}\\ \cline{2-11}
model &  \small{4} &  \small{10} &  \small{30} &  \small{91} &  \small{280} &  \small{865} &  \small{2667} &  \small{5334} &  \small{8000} &  \small{9741} \\
\midrule
base  &       29.1 &        30.6 &        29.2 &        41.5 &         46.4 &         49.7 &          55.1 &          59.3 &          60.9 &          60.8 \\
large &       19.9 &        35.1 &        45.6 &        53.6 &         58.3 &         63.2 &          66.3 &          70.8 &          71.4 &          72.0 \\
small &       20.5 &        23.1 &        19.2 &        26.4 &         25.4 &         24.9 &          32.0 &          36.8 &          40.0 &          42.1 \\
\bottomrule
\end{tabular}
