# Supplementary material for: UNICORN on RAINBOW: A Universal Commonsense Reasoning Model on a New Multitask Benchmark
Source: arXiv:2103.13009 source file (2021-03-24)
Supplement: Supplementary file 3 [file all.multiset_full-tasks.tex]

\begin{tabular}{lllrrrrrr}
\toprule
 & & &\multicolumn{6}{c}{\small{Task}}\\ \cline{4-9}
multiset & knowledge & direction &  \small{\anli{}} &  \small{\cosmosqa{}} &  \small{\hellaswag{}} &  \small{\physicaliqa{}} &  \small{\socialiqa{}} &  \small{\winogrande{}} \\
\midrule
\multirow{9}{*}{\none{}} & \multirow{3}{*}{\atomic{}} & backward &             78.3 &                 81.8 &                  82.5 &                    79.5 &                  74.3 &                   76.9 \\
           &             & bidirectional &             77.9 &                 81.0 &                  82.8 &                    79.3 &                  75.0 &                   78.2 \\
           &             & forward &             77.7 &                 81.0 &                  82.4 &                    79.9 &                  74.4 &                   76.8 \\
\cline{2-9}
           & \multirow{3}{*}{\conceptnet{}} & backward &             78.0 &                 81.8 &                  82.5 &                    79.4 &                  74.3 &                   76.3 \\
           &             & bidirectional &             77.8 &                 81.5 &                  82.3 &                    80.5 &                  74.1 &                   76.3 \\
           &             & forward &             77.5 &                 81.6 &                  82.1 &                    80.0 &                  73.7 &                   76.2 \\
\cline{2-9}
           & \multirow{3}{*}{\together{}} & backward &             78.0 &                 81.2 &                  82.4 &                    81.1 &                  74.4 &                   75.7 \\
           &             & bidirectional &             77.6 &                 81.0 &                  82.6 &                    80.1 &                  74.7 &                   76.4 \\
           &             & forward &             77.5 &                 81.8 &                  82.7 &                    79.8 &                  74.8 &                   76.6 \\
\cline{1-9}
\cline{2-9}
\multirow{9}{*}{\rainbow{}} & \multirow{3}{*}{\atomic{}} & backward &             78.3 &                 81.4 &                  81.3 &                    80.5 &                  75.0 &                   73.2 \\
           &             & bidirectional &             77.7 &                 81.4 &                  81.2 &                    80.4 &                  74.9 &                   71.5 \\
           &             & forward &             77.9 &                 81.3 &                  81.6 &                    80.4 &                  75.0 &                   73.6 \\
\cline{2-9}
           & \multirow{3}{*}{\conceptnet{}} & backward &             78.7 &                 81.8 &                  81.6 &                    81.3 &                  75.0 &                   73.5 \\
           &             & bidirectional &             78.8 &                 80.6 &                  81.5 &                    81.0 &                  74.7 &                   72.9 \\
           &             & forward &             78.3 &                 81.6 &                  81.3 &                    80.6 &                  75.5 &                   73.4 \\
\cline{2-9}
           & \multirow{3}{*}{\together{}} & backward &             77.1 &                 80.9 &                  81.6 &                    81.2 &                  74.3 &                   71.6 \\
           &             & bidirectional &             76.9 &                 81.4 &                  81.0 &                    80.3 &                  75.0 &                   72.2 \\
           &             & forward &             77.7 &                 81.9 &                  81.7 &                    80.8 &                  74.8 &                   72.1 \\
\bottomrule
\end{tabular}
