# Supplementary material for: UNICORN on RAINBOW: A Universal Commonsense Reasoning Model on a New Multitask Benchmark
Source: arXiv:2103.13009 source file (2021-03-24)
Supplement: Supplementary file 4 [file all.single-task_full-tasks.tex]

\begin{tabular}{lrrrrrr}
\toprule
 &\multicolumn{6}{c}{\small{Task}}\\ \cline{2-7}
model &  \small{\anli{}} &  \small{\cosmosqa{}} &  \small{\hellaswag{}} &  \small{\physicaliqa{}} &  \small{\socialiqa{}} &  \small{\winogrande{}} \\
\midrule
large &             77.8 &                 81.9 &                  82.8 &                    80.2 &                  73.8 &                   77.0 \\
\bottomrule
\end{tabular}
