# Supplementary material for: UNICORN on RAINBOW: A Universal Commonsense Reasoning Model on a New Multitask Benchmark
Source: arXiv:2103.13009 source file (2021-03-24)
Supplement: Supplementary file 5 [file all.single-task_learning-curves.tex]

\begin{tabular}{lrrrrrrrrrrrr}
\toprule
 &\multicolumn{12}{c}{\small{Size}}\\ \cline{2-13}
task           &  \small{4} &  \small{10} &  \small{30} &  \small{91} &  \small{280} &  \small{865} &  \small{2667} &  \small{5334} &  \small{8000} &  \small{10667} &  \small{13334} &  \small{16000} \\
\midrule
\anli{}        &       49.2 &        53.1 &        54.8 &        61.1 &         65.6 &         68.4 &          72.3 &          72.1 &          76.1 &           73.4 &           74.4 &           74.9 \\
\cosmosqa{}    &       24.6 &        31.0 &        26.2 &        31.9 &         43.0 &         61.3 &          71.7 &          75.6 &          76.6 &           79.2 &           80.0 &           79.6 \\
\hellaswag{}   &       24.6 &        26.6 &        26.0 &        32.6 &         48.6 &         64.6 &          72.5 &          75.8 &          77.5 &           78.2 &           79.2 &           80.0 \\
\physicaliqa{} &       50.1 &        50.7 &        51.7 &        52.8 &         52.7 &         59.8 &          70.7 &          76.3 &          77.0 &           78.4 &           80.0 &           80.0 \\
\socialiqa{}   &       33.6 &        34.7 &        34.4 &        34.7 &         35.3 &         54.0 &          66.4 &          64.7 &          68.6 &           70.6 &           70.9 &           71.0 \\
\winogrande{}  &       50.1 &        50.7 &        52.9 &        50.7 &         51.1 &         57.9 &          64.2 &          67.4 &          69.9 &           71.4 &           72.2 &           73.1 \\
\bottomrule
\end{tabular}
