# Supplementary material for: UNICORN on RAINBOW: A Universal Commonsense Reasoning Model on a New Multitask Benchmark
Source: arXiv:2103.13009 source file (2021-03-24)
Supplement: Supplementary file 6 [file all.multiset_full-tasks.tex]

\begin{tabular}{llrrrrrr}
\toprule
 & &\multicolumn{6}{c}{\small{Task}}\\ \cline{3-8}
multiset & transfer &  \small{\anli{}} &  \small{\cosmosqa{}} &  \small{\hellaswag{}} &  \small{\physicaliqa{}} &  \small{\socialiqa{}} &  \small{\winogrande{}} \\
\midrule
\multirow{3}{*}{\glue{}} & fine-tune &             78.5 &                 82.4 &                  82.9 &                    80.1 &                  74.3 &                   78.4 \\
             & multitask &             77.2 &                 80.8 &                  81.8 &                    77.6 &                  74.7 &                   76.0 \\
             & sequential &             78.5 &                 81.4 &                  82.3 &                    80.8 &                  74.3 &                   77.9 \\
\cline{1-8}
\multirow{3}{*}{\rainbow{}} & fine-tune &             79.2 &                 82.6 &                  83.1 &                    82.2 &                  75.2 &                   78.2 \\
             & multitask &             78.4 &                 81.1 &                  81.3 &                    80.7 &                  74.8 &                   72.1 \\
             & sequential &             79.5 &                 83.2 &                  83.0 &                    82.2 &                  75.5 &                   78.7 \\
\cline{1-8}
\multirow{3}{*}{\superglue{}} & fine-tune &             78.5 &                 81.7 &                  82.8 &                    80.0 &                  74.7 &                   78.5 \\
             & multitask &             77.7 &                 78.9 &                  80.5 &                    70.7 &                  72.3 &                   69.8 \\
             & sequential &             79.1 &                 82.2 &                  82.5 &                    80.7 &                  74.6 &                   77.6 \\
\bottomrule
\end{tabular}
