# Supplementary material for: UNICORN on RAINBOW: A Universal Commonsense Reasoning Model on a New Multitask Benchmark
Source: arXiv:2103.13009 source file (2021-03-24)
Supplement: Supplementary file 7 [file anli.multiset_learning-curves.tex]

\begin{tabular}{llrrrrrrrrrrrr}
\toprule
 & &\multicolumn{12}{c}{\small{Size}}\\ \cline{3-14}
multiset & transfer &  \small{4} &  \small{10} &  \small{30} &  \small{91} &  \small{280} &  \small{865} &  \small{2667} &  \small{5334} &  \small{8000} &  \small{10667} &  \small{13334} &  \small{16000} \\
\midrule
\multirow{3}{*}{\glue{}} & fine-tune &       49.2 &        53.7 &        60.1 &        61.9 &         66.2 &         69.2 &          72.6 &          72.7 &          75.4 &           73.2 &           74.2 &           74.6 \\
             & multitask &       49.2 &        53.3 &        59.3 &        61.7 &         66.1 &         69.5 &          72.3 &          72.4 &          74.5 &           73.2 &           74.2 &           74.3 \\
             & sequential &       49.1 &        57.1 &        63.1 &        63.8 &         67.4 &         70.0 &          72.8 &          73.4 &          75.8 &           74.3 &           74.3 &           75.4 \\
\cline{1-14}
\multirow{3}{*}{\rainbow{}} & fine-tune &       61.0 &        63.4 &        69.6 &        71.3 &         72.6 &         73.9 &          76.6 &          75.8 &          76.7 &           75.8 &           76.4 &           76.7 \\
             & multitask &       61.9 &        62.9 &        69.6 &        71.4 &         73.0 &         74.3 &          76.4 &          76.7 &          76.9 &           76.8 &           77.5 &           77.2 \\
             & sequential &       61.4 &        65.3 &        70.9 &        71.0 &         73.6 &         73.8 &          75.8 &          75.7 &          76.6 &           76.6 &           76.6 &           76.5 \\
\cline{1-14}
\multirow{3}{*}{\superglue{}} & fine-tune &       49.1 &        57.0 &        59.9 &        63.6 &         66.1 &         69.1 &          71.3 &          71.9 &          75.3 &           73.6 &           73.3 &           74.5 \\
             & multitask &       49.1 &        57.0 &        59.5 &        63.7 &         65.5 &         67.9 &          71.3 &          71.6 &          74.3 &           72.8 &           72.7 &           74.5 \\
             & sequential &       49.2 &        61.5 &        62.6 &        64.8 &         66.3 &         70.2 &          72.2 &          72.3 &          76.1 &           73.6 &           74.0 &           75.2 \\
\bottomrule
\end{tabular}
