# Supplementary material for: UNICORN on RAINBOW: A Universal Commonsense Reasoning Model on a New Multitask Benchmark
Source: arXiv:2103.13009 source file (2021-03-24)
Supplement: Supplementary file 8 [file cosmosqa.multiset_learning-curves.tex]

\begin{tabular}{llrrrrrrrrrrrr}
\toprule
 & &\multicolumn{12}{c}{\small{Size}}\\ \cline{3-14}
multiset & transfer &  \small{4} &  \small{10} &  \small{30} &  \small{91} &  \small{280} &  \small{865} &  \small{2667} &  \small{5334} &  \small{8000} &  \small{10667} &  \small{13334} &  \small{16000} \\
\midrule
\multirow{3}{*}{\glue{}} & fine-tune &       24.5 &        32.4 &        26.0 &        29.3 &         41.5 &         60.7 &          71.9 &          75.7 &          76.3 &           78.6 &           79.8 &           80.1 \\
             & multitask &       24.7 &        32.4 &        26.2 &        29.1 &         41.4 &         59.8 &          71.5 &          75.5 &          76.1 &           77.8 &           78.9 &           79.0 \\
             & sequential &       24.5 &        28.2 &        25.4 &        27.2 &         33.1 &         59.8 &          71.5 &          75.5 &          77.3 &           79.0 &           79.4 &           79.8 \\
\cline{1-14}
\multirow{3}{*}{\rainbow{}} & fine-tune &       54.9 &        61.9 &        57.4 &        60.9 &         62.1 &         67.4 &          74.7 &          78.2 &          79.1 &           80.1 &           81.2 &           81.3 \\
             & multitask &       53.3 &        61.8 &        57.7 &        61.4 &         62.5 &         66.3 &          74.6 &          76.9 &          77.8 &           77.3 &           80.0 &           80.6 \\
             & sequential &       58.2 &        60.1 &        57.7 &        61.6 &         65.0 &         68.7 &          76.4 &          78.1 &          78.7 &           80.2 &           80.1 &           80.5 \\
\cline{1-14}
\multirow{3}{*}{\superglue{}} & fine-tune &       24.6 &        35.3 &        26.0 &        41.5 &         46.4 &         61.0 &          70.6 &          75.6 &          76.7 &           78.8 &           79.9 &           80.5 \\
             & multitask &       24.6 &        34.4 &        26.0 &        40.6 &         44.8 &         60.3 &          70.9 &          74.4 &          75.4 &           77.8 &           77.9 &           78.8 \\
             & sequential &       26.4 &        38.0 &        33.6 &        50.1 &         49.3 &         60.4 &          71.3 &          75.2 &          75.6 &           78.3 &           80.0 &           80.0 \\
\bottomrule
\end{tabular}
