# Supplementary material for: UNICORN on RAINBOW: A Universal Commonsense Reasoning Model on a New Multitask Benchmark
Source: arXiv:2103.13009 source file (2021-03-24)
Supplement: Supplementary file 9 [file hellaswag.multiset_learning-curves.tex]

\begin{tabular}{llrrrrrrrrrrrr}
\toprule
 & &\multicolumn{12}{c}{\small{Size}}\\ \cline{3-14}
multiset & transfer &  \small{4} &  \small{10} &  \small{30} &  \small{91} &  \small{280} &  \small{865} &  \small{2667} &  \small{5334} &  \small{8000} &  \small{10667} &  \small{13334} &  \small{16000} \\
\midrule
\multirow{3}{*}{\glue{}} & fine-tune &       25.3 &        26.4 &        26.7 &        35.3 &         50.2 &         64.3 &          72.7 &          75.2 &          77.0 &           77.9 &           78.8 &           79.6 \\
             & multitask &       25.1 &        26.4 &        26.8 &        36.0 &         49.3 &         63.8 &          72.1 &          75.1 &          76.9 &           77.3 &           78.2 &           78.9 \\
             & sequential &       26.1 &        26.3 &        27.0 &        33.3 &         39.8 &         64.6 &          72.7 &          75.4 &          77.1 &           77.7 &           78.8 &           79.7 \\
\cline{1-14}
\multirow{3}{*}{\rainbow{}} & fine-tune &       53.7 &        49.1 &        47.0 &        55.4 &         63.3 &         67.0 &          74.0 &          76.4 &          77.9 &           78.3 &           79.7 &           80.2 \\
             & multitask &       53.8 &        50.0 &        46.5 &        54.3 &         62.4 &         66.2 &          73.0 &          76.0 &          77.1 &           77.8 &           78.8 &           79.7 \\
             & sequential &       51.6 &        50.8 &        54.4 &        60.1 &         65.8 &         69.2 &          74.7 &          76.3 &          78.3 &           78.4 &           79.8 &           80.2 \\
\cline{1-14}
\multirow{3}{*}{\superglue{}} & fine-tune &       24.2 &        26.4 &        25.8 &        36.1 &         49.6 &         64.7 &          72.4 &          75.2 &          77.1 &           77.8 &           78.7 &           79.6 \\
             & multitask &       25.3 &        26.5 &        25.9 &        35.1 &         48.0 &         63.3 &          71.5 &          74.4 &          76.5 &           77.0 &           77.4 &           78.9 \\
             & sequential &       25.8 &        26.9 &        27.0 &        42.1 &         54.9 &         63.8 &          72.2 &          75.3 &          76.9 &           77.7 &           78.8 &           79.7 \\
\bottomrule
\end{tabular}
