# Supplementary material for: UNICORN on RAINBOW: A Universal Commonsense Reasoning Model on a New Multitask Benchmark
Source: arXiv:2103.13009 source file (2021-03-24)
Supplement: Supplementary file 10 [file physicaliqa.multiset_learning-curves.tex]

\begin{tabular}{llrrrrrrrrrrrr}
\toprule
 & &\multicolumn{12}{c}{\small{Size}}\\ \cline{3-14}
multiset & transfer &  \small{4} &  \small{10} &  \small{30} &  \small{91} &  \small{280} &  \small{865} &  \small{2667} &  \small{5334} &  \small{8000} &  \small{10667} &  \small{13334} &  \small{16000} \\
\midrule
\multirow{3}{*}{\glue{}} & fine-tune &       50.3 &        49.8 &        53.5 &        52.8 &         53.3 &         53.8 &          70.3 &          75.0 &          77.0 &           77.4 &           79.4 &           79.9 \\
             & multitask &       50.3 &        49.6 &        53.8 &        52.7 &         53.6 &         53.4 &          69.5 &          74.0 &          75.5 &           76.0 &           77.6 &           78.9 \\
             & sequential &       50.3 &        49.8 &        53.2 &        51.9 &         56.8 &         59.7 &          71.2 &          74.9 &          77.4 &           78.3 &           79.3 &           80.6 \\
\cline{1-14}
\multirow{3}{*}{\rainbow{}} & fine-tune &       49.0 &        49.7 &        48.5 &        50.5 &         69.1 &         73.2 &          76.5 &          79.0 &          79.4 &           80.3 &           81.8 &           81.8 \\
             & multitask &       49.9 &        49.9 &        51.0 &        50.4 &         68.8 &         73.6 &          76.2 &          78.3 &          78.2 &           79.7 &           80.6 &           80.4 \\
             & sequential &       49.0 &        45.3 &        41.6 &        73.1 &         74.3 &         74.8 &          78.2 &          78.3 &          80.0 &           80.7 &           81.7 &           82.5 \\
\cline{1-14}
\multirow{3}{*}{\superglue{}} & fine-tune &       50.0 &        49.6 &        53.3 &        52.3 &         51.0 &         54.1 &          69.0 &          73.9 &          76.6 &           77.9 &           79.9 &           80.1 \\
             & multitask &       50.1 &        49.6 &        53.6 &        52.4 &         51.2 &         54.5 &          67.2 &          71.2 &          73.5 &           71.8 &           75.8 &           75.4 \\
             & sequential &       50.0 &        49.7 &        53.0 &        52.2 &         51.6 &         50.8 &          69.9 &          75.5 &          77.1 &           78.6 &           78.9 &           80.9 \\
\bottomrule
\end{tabular}
