# Supplementary material for: UNICORN on RAINBOW: A Universal Commonsense Reasoning Model on a New Multitask Benchmark
Source: arXiv:2103.13009 source file (2021-03-24)
Supplement: Supplementary file 11 [file socialiqa.multiset_learning-curves.tex]

\begin{tabular}{llrrrrrrrrrrrr}
\toprule
 & &\multicolumn{12}{c}{\small{Size}}\\ \cline{3-14}
multiset & transfer &  \small{4} &  \small{10} &  \small{30} &  \small{91} &  \small{280} &  \small{865} &  \small{2667} &  \small{5334} &  \small{8000} &  \small{10667} &  \small{13334} &  \small{16000} \\
\midrule
\multirow{3}{*}{\glue{}} & fine-tune &       33.6 &        34.1 &        35.2 &        35.1 &         34.4 &         48.1 &          66.6 &          67.5 &          68.7 &           71.8 &           71.2 &           72.8 \\
             & multitask &       33.6 &        34.7 &        35.2 &        34.9 &         34.8 &         47.0 &          61.6 &          67.5 &          67.7 &           70.8 &           70.4 &           72.0 \\
             & sequential &       33.6 &        34.6 &        34.1 &        35.1 &         35.9 &         53.5 &          68.4 &          68.2 &          70.1 &           71.0 &           72.9 &           72.4 \\
\cline{1-14}
\multirow{3}{*}{\rainbow{}} & fine-tune &       33.6 &        48.2 &        58.1 &        63.9 &         64.7 &         66.6 &          70.2 &          70.6 &          73.1 &           72.7 &           73.6 &           73.6 \\
             & multitask &       33.6 &        50.7 &        58.1 &        64.3 &         65.3 &         67.0 &          69.7 &          70.6 &          72.0 &           72.5 &           73.5 &           73.4 \\
             & sequential &       33.6 &        65.0 &        64.2 &        65.2 &         67.1 &         67.8 &          70.1 &          70.6 &          71.5 &           72.8 &           74.1 &           73.9 \\
\cline{1-14}
\multirow{3}{*}{\superglue{}} & fine-tune &       33.6 &        34.1 &        34.1 &        35.2 &         34.9 &         58.1 &          67.7 &          67.6 &          70.2 &           71.6 &           72.3 &           72.4 \\
             & multitask &       33.6 &        34.7 &        34.6 &        35.2 &         35.4 &         57.3 &          66.3 &          66.7 &          69.7 &           70.5 &           70.0 &           70.9 \\
             & sequential &       33.6 &        34.1 &        34.6 &        34.6 &         35.9 &         58.9 &          67.0 &          68.7 &          69.4 &           71.8 &           72.2 &           72.6 \\
\bottomrule
\end{tabular}
