# Supplementary material for: UNICORN on RAINBOW: A Universal Commonsense Reasoning Model on a New Multitask Benchmark
Source: arXiv:2103.13009 source file (2021-03-24)
Supplement: Supplementary file 12 [file winogrande.multiset_learning-curves.tex]

\begin{tabular}{llrrrrrrrrrrrr}
\toprule
 & &\multicolumn{12}{c}{\small{Size}}\\ \cline{3-14}
multiset & transfer &  \small{4} &  \small{10} &  \small{30} &  \small{91} &  \small{280} &  \small{865} &  \small{2667} &  \small{5334} &  \small{8000} &  \small{10667} &  \small{13334} &  \small{16000} \\
\midrule
\multirow{3}{*}{\glue{}} & fine-tune &       48.5 &        50.5 &        52.3 &        50.4 &         51.5 &         59.4 &          64.8 &          67.2 &          69.9 &           71.3 &           72.5 &           74.2 \\
             & multitask &       49.2 &        50.8 &        51.9 &        51.7 &         51.7 &         59.5 &          63.8 &          66.1 &          68.7 &           69.4 &           71.0 &           71.7 \\
             & sequential &       48.6 &        50.5 &        52.3 &        49.9 &         52.2 &         58.8 &          65.4 &          67.2 &          69.6 &           71.1 &           72.8 &           73.0 \\
\cline{1-14}
\multirow{3}{*}{\rainbow{}} & fine-tune &       52.6 &        52.6 &        52.6 &        53.0 &         56.5 &         63.2 &          66.5 &          69.2 &          71.3 &           72.5 &           73.8 &           73.9 \\
             & multitask &       51.8 &        52.7 &        52.9 &        53.5 &         55.8 &         62.6 &          64.9 &          67.9 &          69.4 &           70.1 &           70.6 &           70.3 \\
             & sequential &       51.0 &        53.2 &        54.1 &        54.7 &         58.8 &         63.3 &          66.9 &          68.4 &          70.5 &           72.5 &           73.4 &           74.9 \\
\cline{1-14}
\multirow{3}{*}{\superglue{}} & fine-tune &       49.3 &        50.7 &        52.2 &        50.7 &         52.9 &         61.7 &          65.2 &          67.2 &          70.1 &           72.1 &           73.5 &           73.5 \\
             & multitask &       50.7 &        50.7 &        52.1 &        51.6 &         52.2 &         60.1 &          64.3 &          64.9 &          68.0 &           68.5 &           70.0 &           69.8 \\
             & sequential &       48.8 &        50.4 &        52.4 &        51.7 &         52.9 &         60.6 &          64.5 &          66.6 &          69.0 &           71.3 &           72.1 &           73.2 \\
\bottomrule
\end{tabular}
